# Supplementary material for: Simplification of Polyhedral Reductions in Practice
Source: arXiv:2411.17498 source file (2024-11-26)
Supplement: Supplementary file 1 [file Appendix.tex]

\appendix

\section{The Example Explained}

We now explain the steps involved in simplifying Eqn.~\ref{eq:MotivatingExample}
repeated below for convenience. \[
Y[i]={\displaystyle \sum_{j=0}^{i}\sum_{k=0}^{i}A[i,j+k]*B[k,j]}\]

First, we introduce a new index variable $l=j+k$ and eliminate $j$. 

This yields ${\displaystyle Y[i]=\sum_{l=0}^{2i}\sum_{\;\; k=\max(0,l-i)\;\;}^{\min(i,l)}A[i,l]*B[k,l-k]}$.
Now, since $A_{i,l}$ is independent of $k$, we use distributivity
to {}``pull it out.''
\[{\displaystyle Y[i]=\sum_{l=0}^{2i}\left(A[i,l]*\sum_{k=\max(0,l-i)}^{\min(i,l)}B[k,l-k]\right)}\].
We introduce a variable $Z[i,l]$ for the result of the inner summation,
so that $Y[i]={\displaystyle \sum_{l=0}^{2i}}A[i,l]*Z[i,l]$ where\\
$\displaystyle Z[i,j]=\sum_{k=\max(0,l-i)}^{\min(i,l)}B[k,l-k]$.
This is simplified to
\[Z[i,l]=\left\{ \begin{array}{rl}
l<i: & {\displaystyle \sum_{k=0}^{l}B[k,l-k]}\\
i\le l: & {\displaystyle \sum_{k=l-i}^{i}B[k,l-k]}\end{array}\right.
\]
where we remove the $\min$ and $\max$ operators in the summation
bounds by separating the $i,l$ space into two regions $i<l$ and
$l\le i$. The complexity of this equation remains cubic (there are
a quadratic number of values of $Z$ to compute, and each one involves
a summation), but once the values of $Z$ are available, $Y$ can
be computed in quadratic time. To simplify the equation for $Z$,
a different technique is needed in each of the two regions.

\textbf{Exploit Reuse:} We identify that in the region $l<i$, the
summation expression is independent of $i$. Hence, we evaluate only
$Z[i,i-1]$ (i.e., on the $l=i-1$ boundary) and then use this value
wherever needed. This will {}``split'' the upper branch into two
sub-branches.

\textbf{Scan Detection:} The second branch of the equation for $Z[i,l]$
has a generalized scan operation. To see it, compare the values of
$Z[i,l]$ and $Z[i-1,l]$ (for $i\leq l$).  We see that
\[{\displaystyle Z[i-1,l]=\sum_{k=l-i+1}^{i-1}B[k,l-k]}\],
which is nothing but the summation that remains if we take 
\[{\displaystyle \sum_{k=l-i}^{i}B[k,l-k]}\]
(i.e., summation for $Z[i,l]$) and remove the first and last terms.
Hence we compute $Z[i,l]$ simply by adding two values to $Z[i-1,l]$,
thus leading to the equations in Figure~\ref{fig:MotivatingExample}~(b)
and the corresponding code in Figure~\ref{fig:MotivatingExample}~(c).
